# Supplementary material for: Survey Design and Estimating Equations when Combining Big Data with Probability Samples
Source: arXiv:2307.11999 source file (2023-08-09)
Supplement: Supplementary file 1 [file supplemental.tex]

%auto-ignore
\pdfoutput=1

% Might need to look at something like
% https://tex.stackexchange.com/questions/463699/proper-reference-numbers-with-subfiles
% so that equation references flow through when producing the standalone version of this
% appendix.

\documentclass[main.tex]{subfiles}

\begin{document}

% Set \wholepaper flag to 1 so that subfiles know that they are being compiled as part of the whole paper, and not as a standalone document.
\renewcommand{\wholepaper}{1}

\doublespacing

\appendix

\setcounter{section}{0}

\subfile{proofs/proofs.tex}

%\bibliographysref{library}

\end{document}
