# Supplementary material for: Survey Design and Estimating Equations when Combining Big Data with Probability Samples
Source: arXiv:2307.11999 source file (2023-08-09)
Supplement: Supplementary file 2 [file supplemental_data_title_page.tex]

%auto-ignore
\pdfoutput=1

\documentclass[main.tex]{subfiles}

\begin{document}

\singlespacing

\begin{titlingpage}

\if0\blind
{
	\renewcommand{\thefootnote}{\fnsymbol{footnote}}
	\title{\papertitle: Supplemental Data}
	\author{\paperauthors}
	\date{\mydate}
	\maketitle
	\footnotetext[1]{\ryanfootnote}
	\footnotetext[2]{\luccafootnote}
	\footnotetext[4]{\mddisclaimer}
	\setcounter{footnote}{0}
	\renewcommand{\thefootnote}{\arabic{footnote}}
} \fi

\end{titlingpage}

\end{document}
